# Supplementary material for: High-throughput screening of small-molecule adsorption in MOF
Source: arXiv:1306.1873 source file (2013-06-08)
Supplement: Supplementary file 1 [file supp.pdf]

# High-throughput screening of small-molecule adsorption in MOF

## — Supplementary Materials —

Pieremanuele Canepa, Calvin A. Arter, Eliot M. Conwill, Daniel H. Johnson, Brian A. Shoemaker, Karim Z. Soliman, and T. Thonhauser

*Department of Physics, Wake Forest University, Winston-Salem, NC 27109, USA.*

(Dated: June 7, 2013)

# I. SIMULATED X-RAY POWDER DIFFRACTION SPECTRA

Figures 1, 2, 3, and 4 depict the simulated X-ray powder diffraction patterns of the four MOF-74-$\mathcal{M}$ with $\mathcal{M}$ = Pd, Os, Ir, and Pr, relevant for their future synthesis.

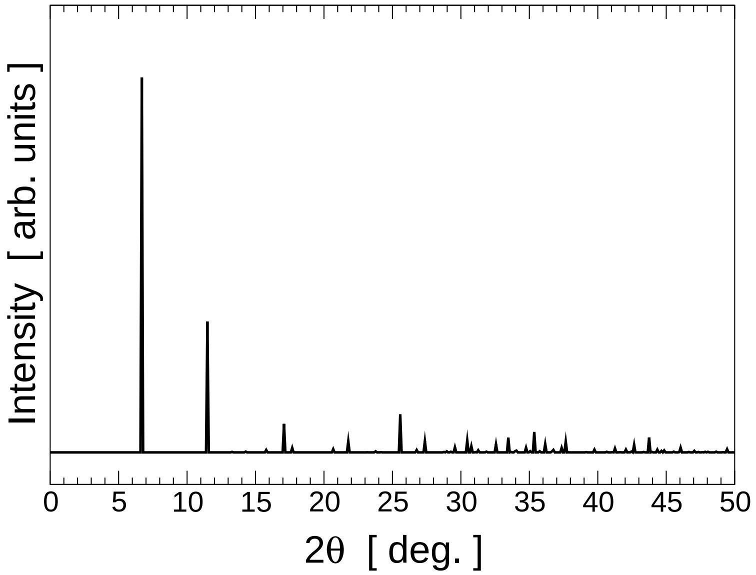


FIG. 1. X-ray powder diffraction pattern for MOF-74-Pd, using a Cu K source.

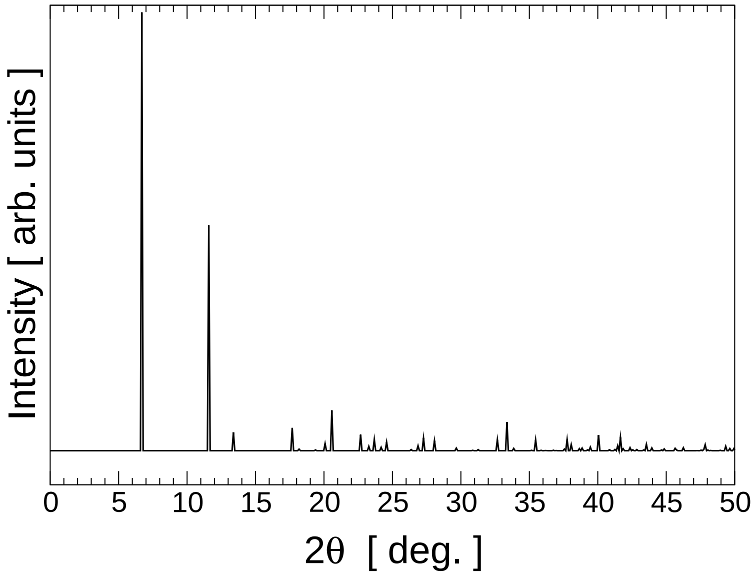


FIG. 2. X-ray powder diffraction pattern for MOF-74-Os, using a Cu K source.

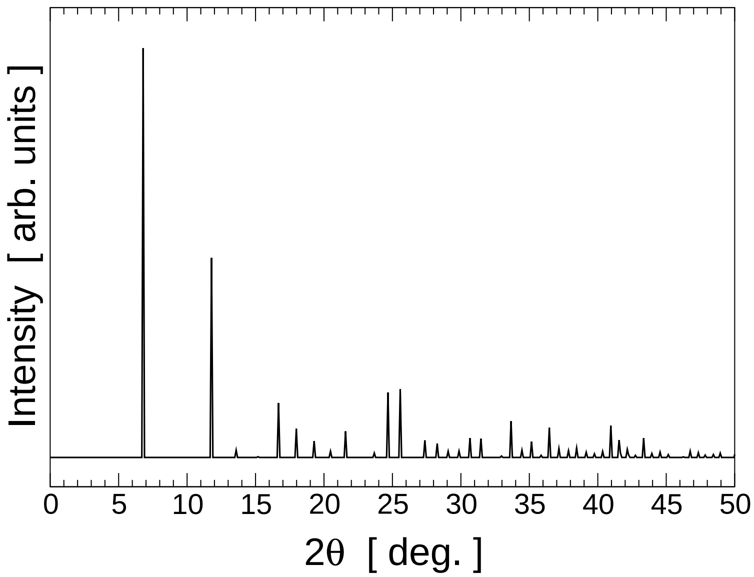


FIG. 3. X-ray powder diffraction pattern for MOF-74-Ir, using a Cu K source.

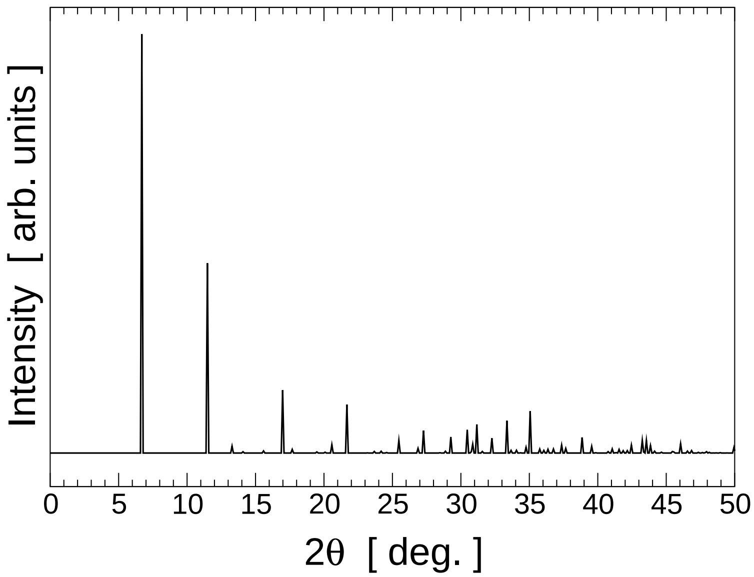


FIG. 4. X-ray powder diffraction pattern for MOF-74-Pt, using a Cu K source.

## II. LATTICE PARAMETERS, INTERATOMIC DISTANCES, ADSORPTION ENERGIES, AND ADSORPTION-ENERGY CONTRIBUTIONS

Table I reports the calculated lattice parameters, relevant atomic distances, adsorption energies, and relevant adsorption-energy contributions for MOF-74-$\mathcal{M}$ with $\mathcal{M}$ = Be, Mg, Al, Ca, Sc, Ti, V, Cr, Mn, Fe, Co, Ni, Cu, Zn, Sr, Zr, Nb, Ru, Rh, Pd, La, W, Os, Ir, and Pt.

Figure 5 shows the molecular aggregation found after full relaxation of MOF-74-$\mathcal{M}$ with $\mathcal{M}$ = Be, Ca, Cr, and Os, once $CO_2$ molecules are adsorbed in the nano-pore. The atom arrangement shown in Fig. 5 clearly demonstrates that the metal ions are not exposed in the pore anymore, inducing a progressive desorption of the adsorbates, which are now agglomerated in the middle of the channel.

Figure 6 clearly shows the chemi-adsorption of $CO_2$ in MOF-74-Al, in which the oxygen of the adsorbate engages the Al species, whereas the C atom of $CO_2$ establishes a strong interaction with the C atoms of the benzene rings (i.e. the linkers). Note that the strong interaction of the C atom of $CO_2$ with the C atoms of the benzene rings disrupts the typical linear symmetry of $CO_2$.

A strong chemi-adsorption is also observed for MOF-74-La in Fig. 7. From this figure we see that $CO_2$ is tightly bound via its oxygen atoms to the La species, introducing a significant structural reconstruction.

TABLE I. Computed lattice constants $a$ and $c$ (in Å) for MOF-74-$\mathcal{M}$ after absorption of six $H_2$, $CO_2$, $CH_4$, and $H_2O$ molecules. Absorption energy $\Delta E$ and deformation energies $\delta E_{\mathrm{MOF}}$ and $\delta E_{\mathrm{M}}$ (in kJ mol$^{-1}$) are also reported. $\mathcal{M}$-X represents the atomic distance (in Å) from the metal ion to the closest atom of the adsorbed molecule.

| | $H_2$ | | | | | | $CO_2$ | | | | | | $CH_4$ | | | | | | $H_2O$ | | | | | |
|---|---|---|---|---|---|---|---|---|---|---|---|---|---|---|---|---|---|---|---|---|---|---|---|---|
| $\mathcal{M}$ | $a$ | $c$ | $\mathcal{M}$-X | $\Delta E$ | $\delta E_{\mathrm{MOF}}$ | $\delta E_{\mathrm{M}}$ | $a$ | $c$ | $\mathcal{M}$-X | $\Delta E$ | $\delta E_{\mathrm{MOF}}$ | $\delta E_{\mathrm{M}}$ | $a$ | $c$ | $\mathcal{M}$-X | $\Delta E$ | $\delta E_{\mathrm{MOF}}$ | $\delta E_{\mathrm{M}}$ | $a$ | $c$ | $\mathcal{M}$-X | $\Delta E$ | $\delta E_{\mathrm{MOF}}$ | $\delta E_{\mathrm{M}}$ |
| Be | 25.518 | 6.774 | 3.311 | –16.5 | 0.4 | –0.8 | 25.413 | 6.649 | 3.778 | –60.2 | 4.2 | –18.1 | 25.413 | 6.649 | 3.544 | –40.2 | 0.9 | –5.8 | 25.187 | 6.671 | 3.835 | –41.4 | 2.3 | –4.0 |
| Mg | 26.056 | 6.897 | 2.853 | –15.8 | 0.3 | –0.7 | 25.944 | 6.852 | 2.398 | –53.4 | 1.2 | –6.0 | 25.944 | 6.852 | 2.648 | –37.0 | 1.3 | –4.6 | 25.943 | 6.870 | 2.232 | –73.2 | 4.2 | –5.0 |
| Al | 25.535 | 6.486 | 2.320 | –19.8 | –0.9 | –0.3 | 24.988 | 6.642 | 1.807 | –118.4 | 126.6 | 207.7 | 25.413 | 6.649 | 2.656 | –38.2 | 1.0 | –4.6 | 25.480 | 6.503 | 2.010 | –135.7 | 23.6 | –1.1 |
| Ca | 25.122 | 7.650 | 3.269 | –18.7 | 1.2 | –0.4 | 24.598 | 7.208 | 2.621 | –57.0 | 1.7 | –10.0 | 25.492 | 7.538 | 2.809 | –40.1 | –5.2 | 0.8 | 26.233 | 7.505 | 2.485 | –87.1 | 9.1 | –2.2 |
| Sc | 23.424 | 7.363 | 3.473 | –19.6 | 0.6 | –0.6 | 23.450 | 7.319 | 3.746 | –53.0 | 1.5 | –8.5 | 23.840 | 7.272 | 2.905 | –45.3 | 1.3 | –7.0 | 25.786 | 7.126 | 2.265 | –113.1 | 16.5 | –0.9 |
| Ti | 21.503 | 7.023 | 3.513 | 1.4 | 12.0 | 8.0 | 22.696 | 7.257 | 4.400 | –49.4 | 5.0 | –12.6 | 22.606 | 7.269 | 3.543 | –39.9 | 5.8 | –9.6 | 22.583 | 7.274 | 4.283 | –50.7 | 6.0 | -35.7 |
| V | 25.417 | 8.135 | 3.471 | –20.0 | –0.6 | –0.4 | 26.026 | 6.827 | 2.257 | –52.7 | 7.5 | –1.0 | 26.007 | 6.934 | 2.378 | –43.3 | 2.4 | –3.2 | 26.038 | 6.900 | 2.185 | –110.9 | 6.1 | –0.9 |
| Cr | 26.206 | 6.308 | 3.767 | –19.8 | 0.2 | –0.5 | 26.053 | 6.529 | 3.826 | –52.9 | 1.0 | –4.4 | 25.987 | 6.500 | 2.975 | –37.8 | 1.2 | –5.9 | 26.955 | 5.802 | 2.499 | –51.1 | 12.4 | –2.4 |
| Mn | 26.316 | 6.928 | 3.400 | –19.0 | 0.5 | –0.3 | 26.170 | 7.064 | 2.755 | –53.7 | 2.6 | –3.6 | 26.170 | 7.064 | 2.694 | –43.2 | 0.5 | –4.9 | 26.244 | 7.011 | 2.341 | –73.1 | 11.3 | –2.7 |
| Fe | 25.994 | 6.810 | 3.461 | –19.8 | –0.2 | –0.4 | 25.854 | 6.639 | 3.705 | –51.2 | 1.4 | –5.4 | 25.854 | 6.639 | 3.131 | –39.8 | 1.5 | –5.9 | 31.031 | 4.128 | 2.142 | –129.7 | 30.1 | –4.0 |
| Co | 26.109 | 7.004 | 3.387 | –19.8 | 0.5 | –0.4 | 25.990 | 6.870 | 2.531 | –45.8 | 1.5 | –5.4 | 25.628 | 6.159 | 2.707 | –37.4 | 0.8 | –5.1 | 26.252 | 6.582 | 2.254 | –71.7 | 12.1 | –3.0 |
| Ni | 25.740 | 5.997 | 3.415 | –19.1 | 0.3 | –1.5 | 25.628 | 6.159 | 2.524 | –47.4 | 0.6 | –6.1 | 25.628 | 6.159 | 3.033 | –36.0 | 0.6 | –6.3 | 26.062 | 5.904 | 2.183 | –60.6 | 3.9 | –3.4 |
| Cu | —[a] | — | — | — | — | — | 25.990 | 6.870 | 2.973 | –42.9 | 0.8 | –0.6 | 26.213 | 6.094 | 2.919 | –39.7 | 0.6 | –5.1 | 30.246 | 4.256 | 2.233 | –90.3 | –18.1 | 8.8 |
| Zn | 26.108 | 6.816 | 2.745 | –20.9 | 0.4 | –2.0 | 26.159 | 6.570 | 3.826 | –52.4 | 1.0 | –3.1 | 26.177 | 6.472 | 2.851 | –44.6 | 1.7 | –5.8 | 26.769 | 5.841 | 2.228 | –75.5 | 3.4 | –3.8 |
| Sr | 27.192 | 6.544 | 3.250 | –18.6 | 1.2 | –0.4 | 27.513 | 6.559 | 2.980 | –49.7 | 5.2 | –1.7 | 26.827 | 6.765 | 2.831 | –43.9 | –0.2 | –5.1 | 30.973 | 4.447 | 2.505 | -153.6 | 31.2 | 0.8 |
| Zr | 23.329 | 7.517 | 3.651 | –17.8 | 0.2 | –0.9 | 23.060 | 7.552 | 4.265 | –52.0 | 1.7 | –11.9 | 22.984 | 7.566 | 3.537 | –43.8 | 2.1 | –8.4 | 23.298 | 7.260 | 2.370 | –90.3 | 29.7 | –3.3 |
| Nb | 26.905 | 3.031 | 2.911 | –20.7 | –0.2 | 0.2 | 27.262 | 6.520 | 2.361 | –89.1 | 5.5 | –0.6 | 26.171 | 6.525 | 2.533 | –44.5 | 4.9 | –1.0 | 27.255 | 6.559 | 2.325 | –124.5 | 3.6 | –1.8 |
| Ru | 27.112 | 6.261 | 3.539 | –20.5 | –0.3 | –0.7 | 27.092 | 5.901 | 3.794 | –49.5 | 1.8 | –2.5 | 27.065 | 5.927 | 3.220 | –38.5 | 1.7 | –3.8 | 25.970 | 4.947 | 3.163 | –77.5 | 15.0 | –0.1 |
| Rh | 25.936 | 7.120 | 3.650 | –20.8 | –0.5 | –0.4 | 25.515 | 6.827 | 3.968 | –52.5 | 1.3 | –7.1 | 25.545 | 6.818 | 2.911 | –36.1 | 1.0 | –6.2 | 25.782 | 6.798 | 3.882[b] | –50.5 | 0.6 | –2.9 |
| Pd | 26.271 | 6.138 | 4.029 | –19.5 | 0.1 | –0.7 | 26.611 | 6.384 | 3.591 | –51.3 | 0.2 | –2.3 | 26.424 | 6.413 | 3.102 | –37.4 | 0.6 | –5.7 | 26.721 | 6.360 | 3.447[b] | –46.1 | 0.7 | –2.6 |
| La | 26.9673 | 7.099 | 2.977 | –20.2 | –0.9 | –0.7 | 27.254 | 6.223 | 2.844 | –90.0 | 6.2 | 6.6 | 26.672 | 6.369 | 2.830 | –40.9 | 0.8 | –4.9 | 27.460 | 5.935 | 2.661 | –105.2 | 17.1 | 0.3 |
| W | 26.777 | 6.336 | 3.126 | –21.9 | –0.9 | –0.4 | 26.926 | 6.134 | 4.030 | –52.0 | 0.5 | –5.2 | 27.052 | 6.204 | 2.172 | –40.8 | 1.7 | –5.6 | 27.126 | 6.281 | 2.231 | –133.2 | 7.9 | 0.2 |
| Os | 26.294 | 6.480 | 4.121 | –19.1 | 0.3 | –10.0 | 26.319 | 4.953 | 4.250 | –58.8 | 1.1 | –16.2 | —[a] | — | — | — | — | — | 26.134 | 4.973 | 3.488[b] | –50.5 | 4.7 | –1.7 |
| Ir | 26.021 | 7.276 | 3.676 | –20.4 | –0.4 | –0.4 | 21.916 | 6.917 | 3.907 | –55.1 | 8.8 | –18.0 | 25.654 | 6.839 | 3.098 | –36.8 | 1.2 | –6.1 | 25.956 | 6.804 | 3.915[b] | –49.0 | 1.2 | –2.8 |
| Pt | 26.597 | 6.351 | 3.790 | –19.3 | –0.4 | –0.6 | 26.527 | 6.468 | 3.966 | –52.2 | 0.2 | –2.5 | 26.276 | 6.541 | 3.237 | –36.1 | 1.0 | –5.9 | 26.623 | 6.471 | 4.239[b] | –45.1 | 1.0 | –2.4 |

[a] Simulation considered not converged since we observe unphysical dissociation due to huge structural strains.

[b] Here we give the distance between the site labeled as 2$^{\mathrm{nd}}$ in Fig. 4 in the main manuscript and the closest atom of the bound molecule.

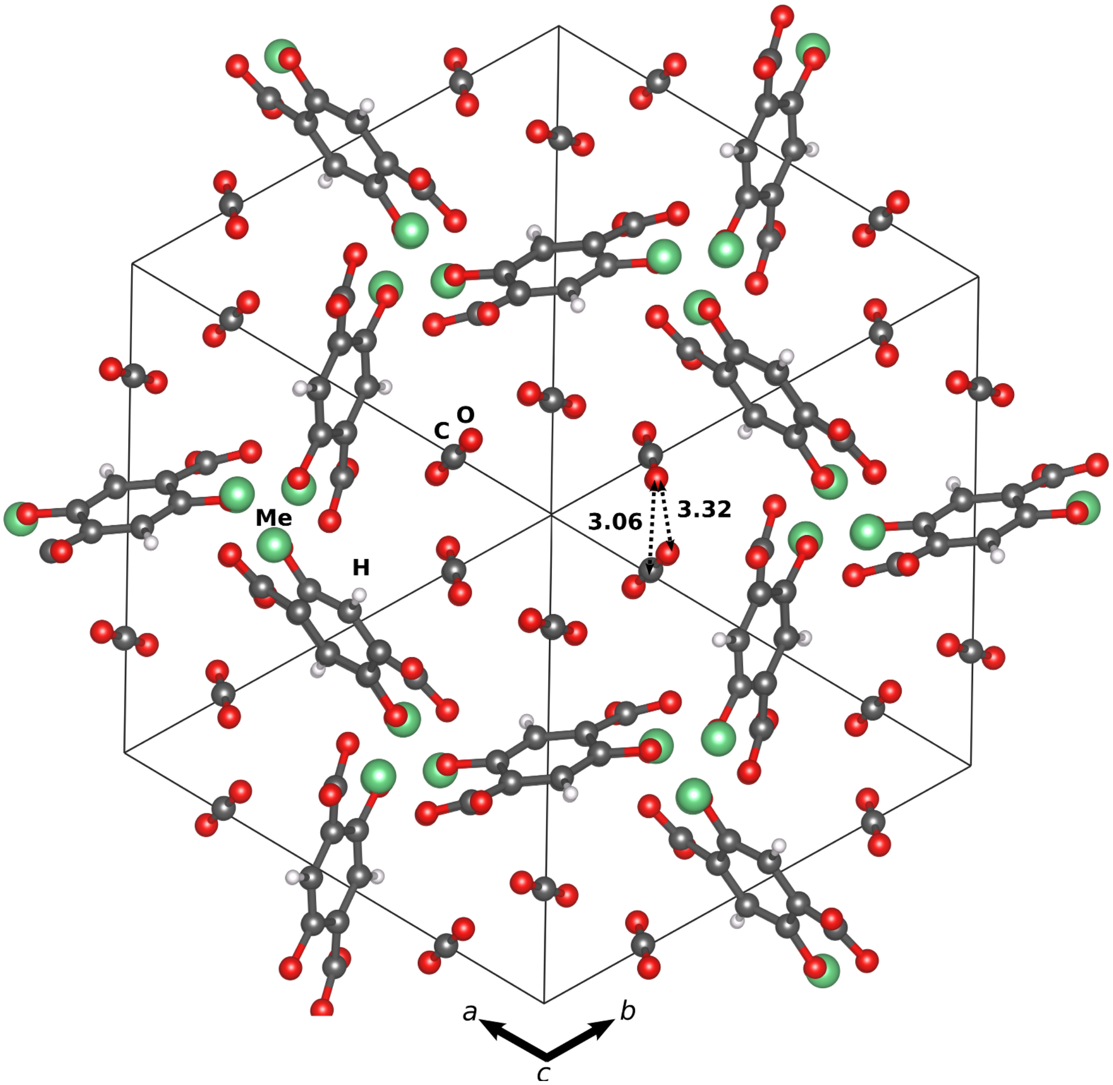


FIG. 5. $CO_2$ absorbed in MOF-74-$\mathcal{M}$ with $\mathcal{M}$ = Be, Ca, Cr, and Os. Bond lengths (in Å), depicted as dashed lines, refer to the case of MOF-74-Be, but are comparable to the other cases.

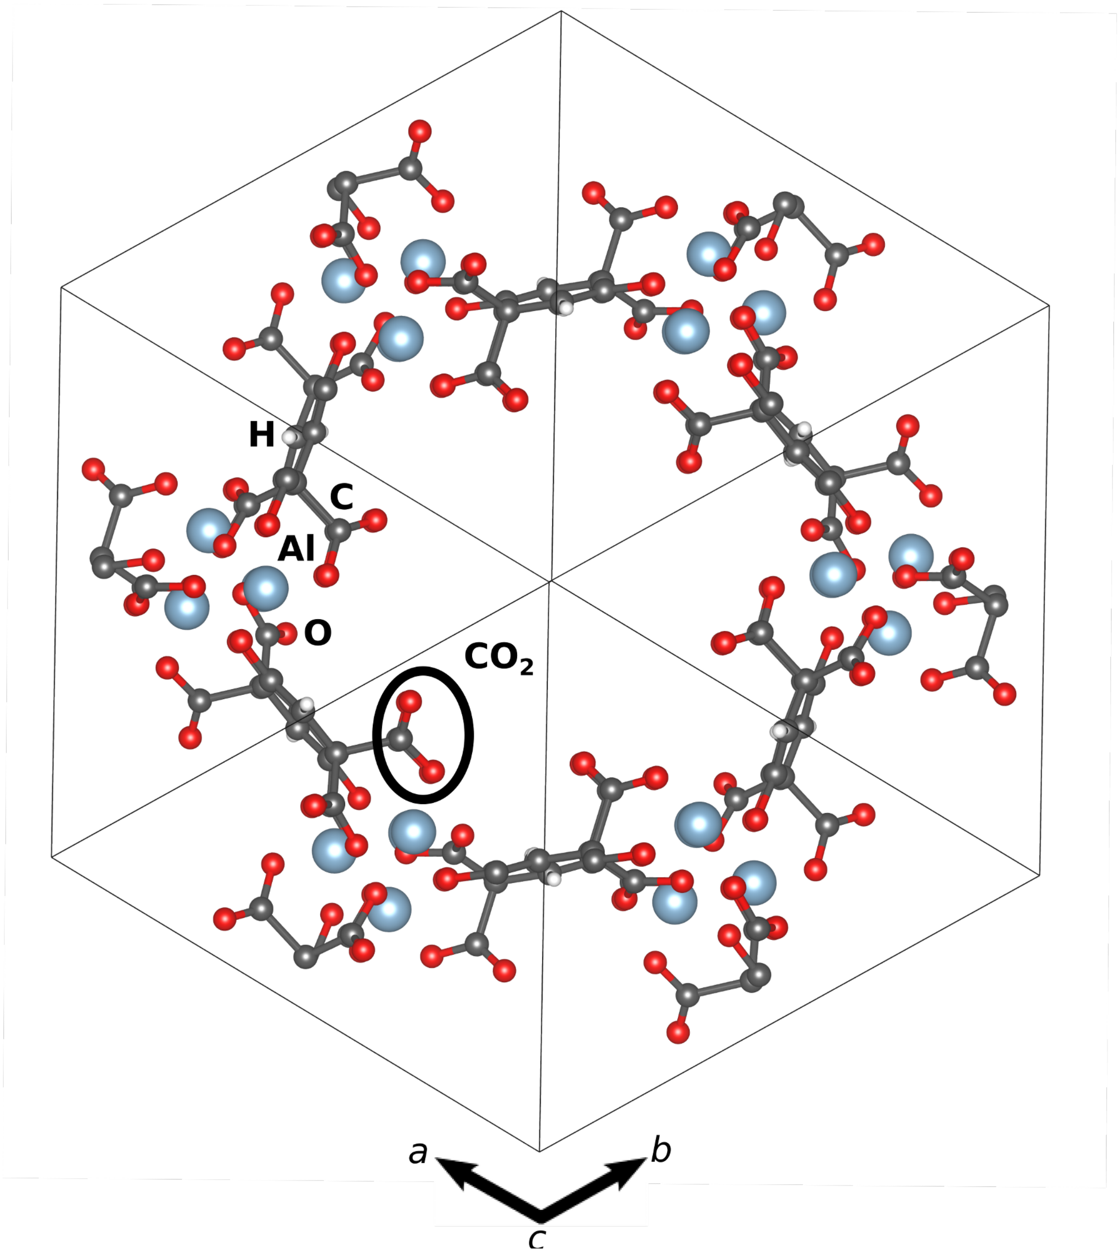


FIG. 6. MOF-74-Al with $CO_2$ adsorbed at all metal sites. Notice the strong deviation of the bound $CO_2$ from its typical linear structure.

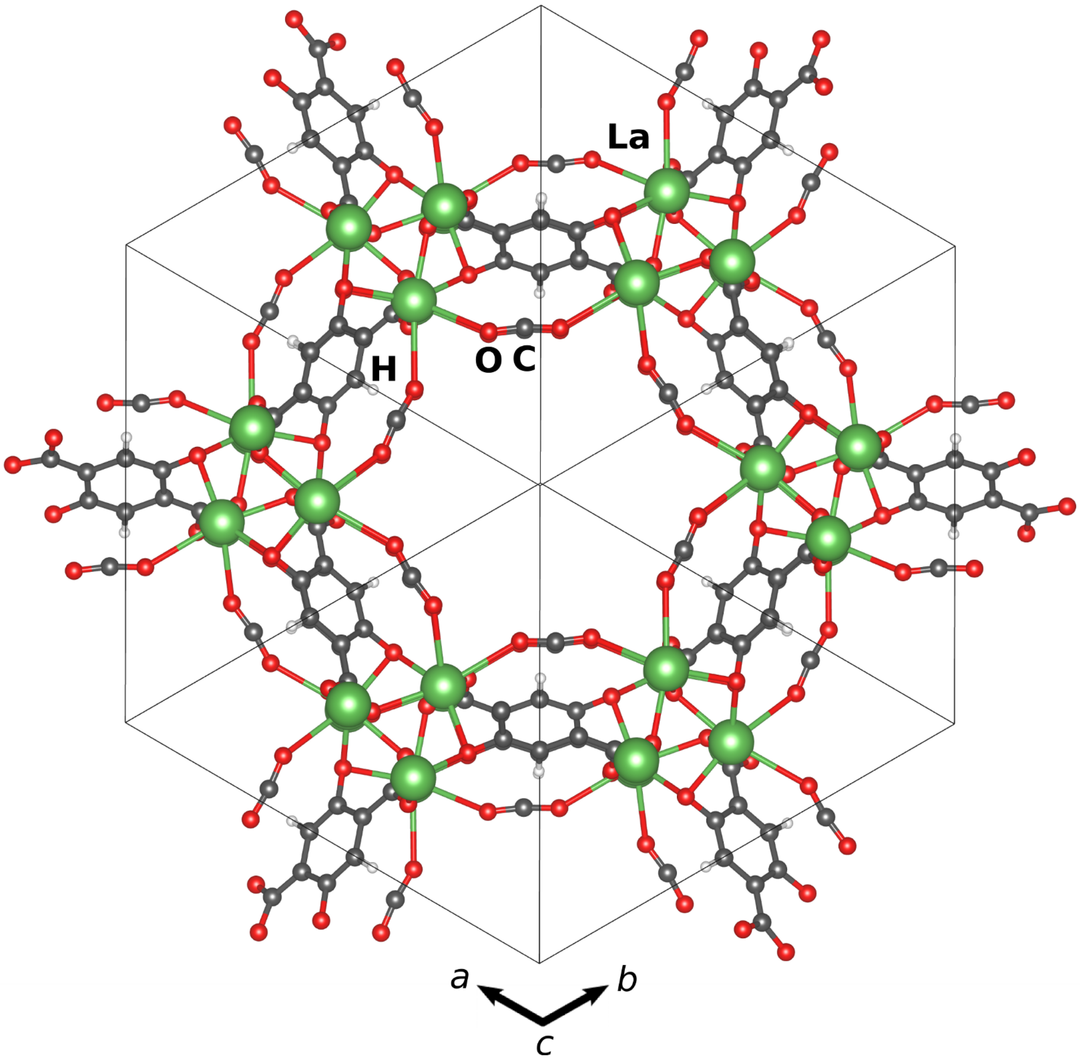


FIG. 7. MOF-74-La with $CO_2$ adsorbed between all metal sites.

## III. DENSITY OF STATES FOR SELECTED CASES OF WATER IN MOF-74-$\mathcal{M}$

Figures 8, 9, 10, 11, and 12 depict the projected density of states (pDOS) of the relevant atoms involved in the chemi-absorption of $H_2O$ in MOF-74-Sc, -Al, -V, -Nb, and -La. In each figure we report only the pDOS of the O and H atoms of $H_2O$, O, and the metal species of MOF-74-$\mathcal{M}$; other atoms are removed for the sake of clarity. Metal states dominate at the Fermi energies of MOF-74-V, -Nb, and -W, as can bee seen in Figs. 10, 11, and 12, demonstrating the metallic nature of some of these materials.

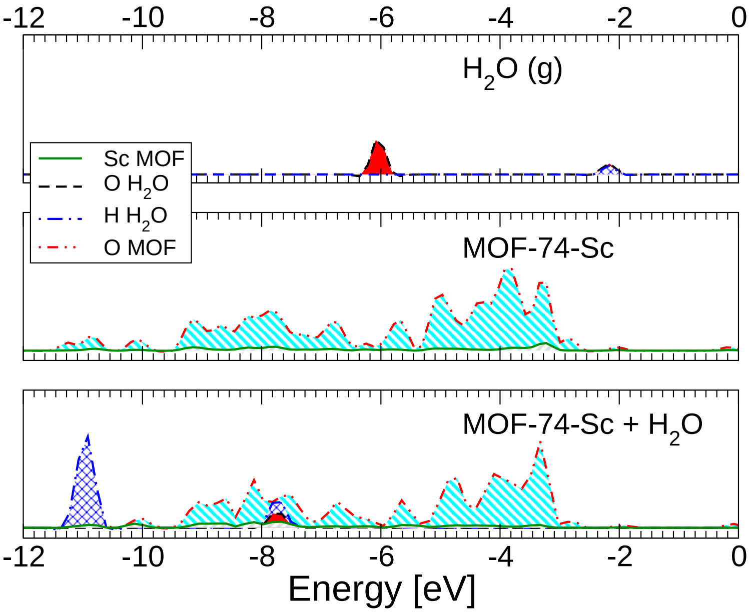


FIG. 8. pDOS for MOF-74-Sc with $H_2O$, MOF-74-Sc, and $H_2O$ in gas phase. Energies are given in eV with respect to the top of the valence band. Note that up- and down-states are added together.

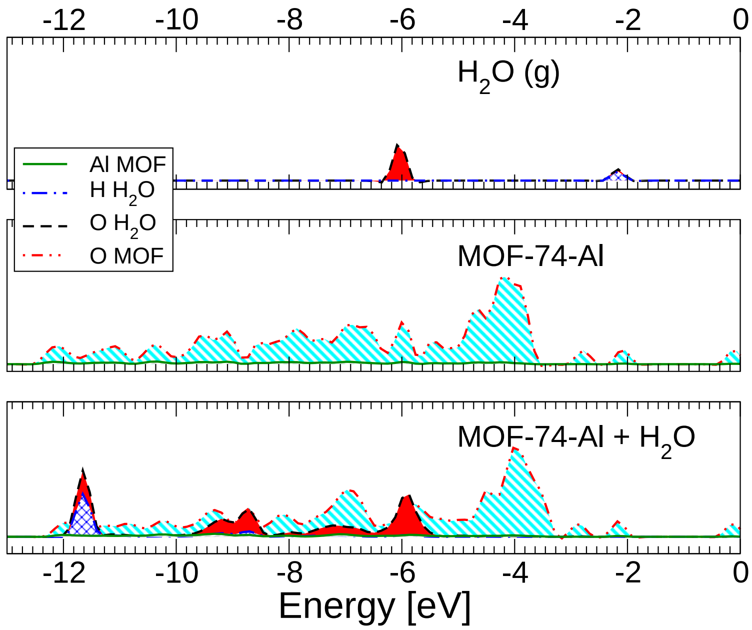


FIG. 9. As in Fig. 8, but here for MOF-74-Al.

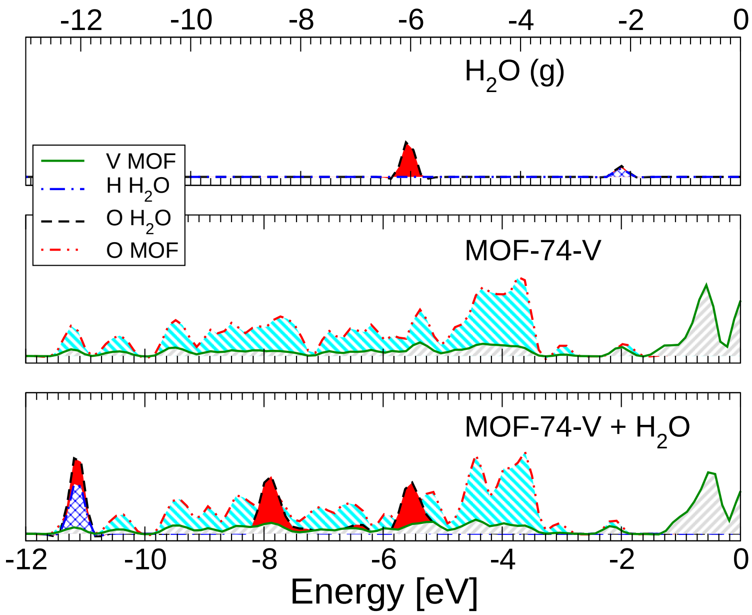


FIG. 10. As in Fig. 8, but here for MOF-74-V.

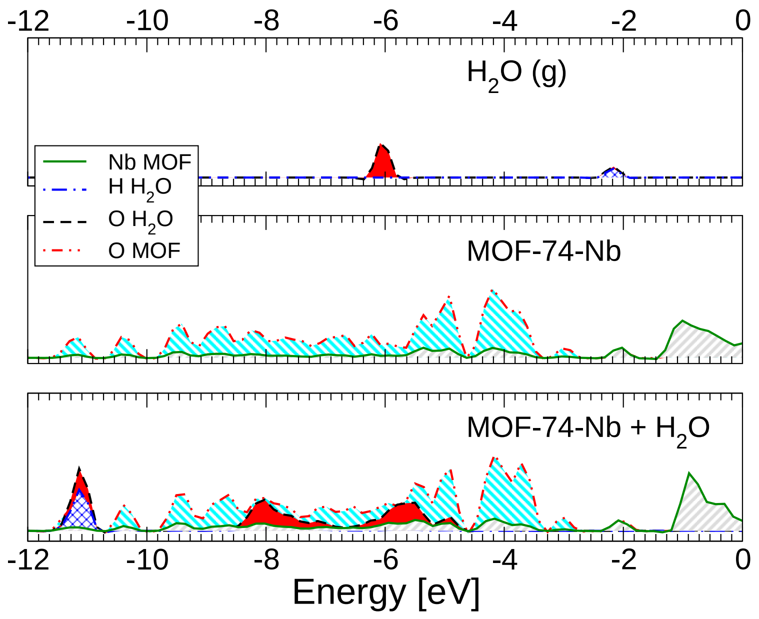


FIG. 11. As in Fig. 8, but here for MOF-74-Nb.

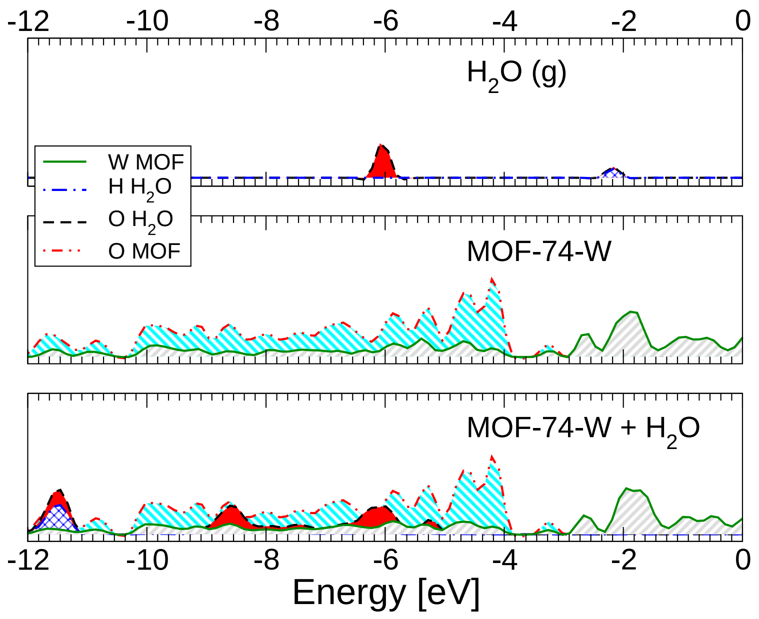


FIG. 12. As in Fig. 8, but here for MOF-74-W.
